# Supplementary material for: Multi-channel Kondo impurity dynamics in a Majorana device
Source: arXiv:1312.3802 source file (2014-08-12)
Supplement: Supplementary file 1 [file SM.pdf]

# Supplementary Material to: Majorana spin dynamics in the topological Kondo effect

A. Altland,[1] B. Beri,[2] R. Egger,[3] and A.M. Tsvelik[4]

[1] *Institut für Theoretische Physik, Universität zu Köln, Zülpicher Str. 77, D-50937 Köln, Germany*
[2] *School of Physics and Astronomy, University of Birmingham, Edgbaston, Birmingham B15 2TT, UK*
[3] *Institut für Theoretische Physik, Heinrich-Heine-Universität, D-40225 Düsseldorf, Germany*
[4] *Department of Condensed Matter Physics and Materials Science, Brookhaven National Laboratory, Upton, NY 11973-5000, USA*

(Dated: August 12, 2014)

We here provide additional results and derivations.

PACS numbers: 71.10.Pm, 72.23.-b, 74.50.+r

## STRONG COUPLING MAJORANA SPIN

In this section, we obtain the most relevant operators arising near the Kondo fixed point in the presence of a 'bare' Zeeman field of the form

$$H_Z^{(lm)} = ih_{lm}\gamma_l\gamma_m. \tag{1}$$

In the main text, the result of this derivation is quoted in Eq. (4). As the product $\gamma_l\gamma_m$ does not commute with all parity products $p_jp_k$, intuitively, one expects Eq. (1) to give rise to processes simultaneously flipping certain parities while tunneling $\tilde{\boldsymbol{\theta}}(0)$ from its original location to one of the minima of the potential corresponding to the new parity configuration. Below we obtain the operators corresponding to such processes from symmetry considerations.

There are several natural requirements: (i) The operators should conserve all the $p_jp_k$ that $H_Z^{lm}$ conserves, but couple those $p_jp_k$ sectors connected by $H_Z^{lm}$. (ii) They should preserve the boundary conditions implied by the Kondo fixed point. In particular, they should not leave the Hilbert space sector where parity products $p_jp_k$ and boson fields $\tilde{\boldsymbol{\theta}}(0)$ conspire to minimize $H_K$ [see Eq. (3) of the main text]. (iii) They should have the same SO($M$) rotational properties as $H_Z^{(lm)}$. (iv) They should commute with the overall fermion parity on the island, $P_{\rm tot} \sim \prod_{j=1}^{M_{\rm tot}}\gamma_j$. (v) They should conserve charge. (vi) They should act at the impurity location $x=0$ only.

Requirements (i) and (ii) express the intuitive tunneling picture more formally. The tunneling of $\tilde{\boldsymbol{\theta}}(0)$ is implemented by exponentials of $\tilde{\boldsymbol{\varphi}}$. The operators we are after will thus contain such exponentials. To elucidate the implications of the third requirement (and make further progress with the others afterwards), it is thus useful to summarize the SO($M$) properties of field exponentials. These come from the bosonization identity (with $L/R$ for left/right movers and $x\le 0$) [1, 2]

$$\psi_{jL}^{(\dagger)}(x) \sim \Gamma_j e^{\pm i\frac{\varphi_j(x)-\theta_j(x)}{2}},\ \psi_{jR}^{(\dagger)}(x) \sim \Gamma_j e^{\pm i\frac{\varphi_j(x)+\theta_j(x)}{2}}, \tag{2}$$

and the fact that electron operators transform in the vector representation, $\psi'_{jL/R}(x) = \sum_l O_{lj}\psi_{lL/R}(x)$, where $O\in$ SO($M$). Rotations are thus defined for combinations of Klein factors and field exponentials. To ensure the correct SO($M$) features, the field exponentials in the sought operators will therefore be also attached to Klein factors. (Since left/right movers for $x\le 0$ can be unfolded into right movers on the full line, there is only one Klein factor shared between a left and a right mover.)

Equation (2) directly provides operators satisfying requirements (i) to (v). As $p_jp_k=\gamma_j\gamma_k\Gamma_j\Gamma_k$, fermion bilinears $\propto \Gamma_l\Gamma_m$ alter $p_jp_k$ the same way as $\gamma_l\gamma_m$, taking care of requirement (i). Decomposing $\boldsymbol{\theta}$ as in the main text,

$$\theta_l(x) = \mathbf{w}_l\cdot\tilde{\boldsymbol{\theta}}(x) + \frac{1}{\sqrt{M}}\theta_0(x), \tag{3}$$

and $\varphi_l$ similarly, with $(\mathbf{w}_l, \frac{1}{\sqrt{M}})$ being the $l$th row of an O($M$) matrix, we also find that any object built out of fermions will satisfy requirement (ii). In fact, whenever $\Gamma_j$ flips $p_j$, the exponential will shift $\tilde{\boldsymbol{\theta}}(0)\to\tilde{\boldsymbol{\theta}}(0)+2\pi\mathbf{w}_j$, which leads to a sign change in $\exp[i(\mathbf{w}_k-\mathbf{w}_j)\tilde{\boldsymbol{\theta}}(0)/2]$, thus keeping $H_K$ minimized. Fermion bilinears of the form $B_{\alpha\beta}^{(lm)}(x) = i[\psi_{l\alpha}^\dagger(x)\psi_{m\beta}(x) - \psi_{m\alpha}^\dagger(x)\psi_{l\beta}(x)]$ (with $\alpha,\beta=L,R$) also satisfy requirements (iii) to (v). Indeed, they trivially fulfill (iv) and (v), and they also have the right SO($M$) properties. For the latter, note that both $\gamma_l\gamma_m$ and $B_{\alpha\beta}^{(lm)}(x)$ can be expressed using the elementary antisymmetric matrix $A^{(lm)}$, i.e., $\gamma_l\gamma_m = \frac{1}{2}\gamma_j A_{jk}^{(lm)}\gamma_k$ and $B_{\alpha\beta}^{(lm)}(x) = \psi_{j\alpha}^\dagger(x)A_{jk}^{(lm)}\psi_{k\beta}(x)$, where we use the summation convention. Noting that the $A_{jk}^{(lm)}$ are SO($M$) generators, as both $\gamma_l$ and $\psi_{l\alpha}^{(\dagger)}$ transform under the vector representation, both bilinears above transform under the adjoint representation.

In order to also fulfil requirement (vi), we consider the boundary limit $x\to 0$ of $B_{\alpha\beta}^{(lm)}(x)$. This leads to the operators

$$\tilde{\mathcal{S}}_{lm}^{(\pm)} \sim i\Gamma_l\Gamma_m e^{i\frac{\mathbf{w}_l\pm\mathbf{w}_m}{2}\tilde{\boldsymbol{\varphi}}(0)} e^{i\frac{\mathbf{w}_l-\mathbf{w}_m}{2}\tilde{\boldsymbol{\theta}}(0)} + \text{h.c.} \tag{4}$$

Here $\tilde{\mathcal{S}}_{lm}^{(-)}$ is the $x\to 0$ limit of the SO($M$) 'spin' density $J_{L/R}^{(lm)} = B_{\alpha\alpha}^{(lm)}$. It is therefore a free-fermion

operator of dimension $\Delta_- = 1$, a marginal perturbation. The operator $\tilde{\mathcal{S}}_{lm}^{(+)}$ arises in the $x \to 0$ limit of $B_{LR}^{(lm)} + B_{LR}^{(lm)\dagger} = B_{LR}^{(lm)} + B_{RL}^{(lm)}$, as numerator of a singular term that diverges as $x^{-2/M}$. This singularity is the consequence of the emergent boundary conditions. Being a fermion bilinear, the overall term has to have unit dimension, from which we find $\Delta_+ = 1-2/M$. This coincides with the dimension of the adjoint primary in terms of the Affleck-Ludwig BCFT [3]. Due to this correspondence and the identical SO($M$) properties, we identify $\tilde{\mathcal{S}}_{lm}^{(+)}$ with this field. This is further supported by the fact that in BCFT, the adjoint primary appears in the same limit of fermion bilinears. The noninteger $\Delta_+$ means that $\tilde{\mathcal{S}}_{lm}^{(+)}$ does not appear in a free fermion theory. As $\Delta_+ < 1$, the adjoint primary is a relevant perturbation.

We can now simplify $\tilde{\mathcal{S}}_{lm}^{(\pm)}$ by using $\Gamma_l \Gamma_m = \gamma_l \gamma_m p_l p_m$. This allows us to separate a factor $p_l p_m \exp[i\frac{\mathbf{w}_l - \mathbf{w}_m}{2}\tilde{\boldsymbol{\theta}}(0)]$, which – being identical to one of the boundary terms in $H_K$ – commutes with all $\Gamma_j \Gamma_k \exp[i\frac{\mathbf{w}_j \pm \mathbf{w}_k}{2}\tilde{\boldsymbol{\varphi}}(0)]$, and evaluates to unity in the Hilbert space implementing the Kondo boundary conditions. Near the Kondo fixed point, therefore, one can equivalently consider

$$\mathcal{S}_{lm}^{(\pm)} \sim i\gamma_l\gamma_m e^{i\frac{\mathbf{w}_l \pm \mathbf{w}_m}{2}\cdot\tilde{\boldsymbol{\varphi}}(0)} + \text{h.c.} \qquad (5)$$

which coincides with Eq. (4) in the main text. Our analysis so far left the phases in the $\mathcal{S}_{lm}^{(+)}$ exponentials unspecified: the logic would be the same for $B_{LR}^{(lm)} \to e^{i\chi_{lm}} B_{LR}^{(lm)}$ with any $\chi_{lm}$. We note in passing that there is no analogous freedom in $B_{\alpha\alpha}^{(lm)}$ since a phase leaves $\mathcal{S}_{lm}^{(-)}$ unaltered apart from its overall normalization. However, requiring a consistent operator algebra (e.g., having three adjoints for $M = 3$) imposes constraints on the phases, ensuring that they enter merely through nonzero overall factors in the correlators considered below. For this reason, we omit them and work with $\mathcal{S}_{lm}^{(+)}$ in Eq. (5) henceforth.

## CORRELATION FUNCTIONS

In this section, we provide details about the Majorana spin ($\mathcal{S}_{lm}^{(+)}$) imaginary-time correlation functions. The boundary field $\tilde{\varphi}_j(0)$ can be viewed as a chiral boson at $x = 0$, with correlations given by [2]

$$\left\langle \mathcal{T}_\tau \prod_j e^{i\mathbf{u}^j\cdot\tilde{\boldsymbol{\varphi}}(\tau_j,0)} \right\rangle \sim \delta_{0,\sum_j \mathbf{u}^j} \prod_{j<k} \frac{1}{|\tau_j - \tau_k|^{-4\mathbf{u}^j\cdot\mathbf{u}^k}}. \qquad (6)$$

Equation (6) contains only the phase exponentials. However, since the time dependence due to $\gamma_j\gamma_k$ products is already fixed by anticommutation rules and $\mathcal{S}_{jk}^{(+)}$ commutes with $H_K$, the entire time evolution of the correlation functions is due to a free boson Hamiltonian.

We first consider the three-point function for $M = 3$. We represent the three independent products $\gamma_k\gamma_l$ via Pauli matrices, $i\varepsilon_{jkl}\gamma_k\gamma_l = \sigma_j$, and use $S_j = \varepsilon_{jkl}\mathcal{S}_{kl}^{(+)}$ as in the main text. The three operators $S_{j=1,2,3}$ are thereby expressed as

$$\begin{aligned} S_{1,2} &\sim \sigma_{1,2} e^{-i\frac{\mathbf{w}_{1,2}}{2}\cdot\tilde{\boldsymbol{\varphi}}(0)} + \text{h.c.}, \\ S_3 &\sim \sigma_3 e^{i\frac{(\mathbf{w}_1+\mathbf{w}_2)}{2}\cdot\tilde{\boldsymbol{\varphi}}(0)} + \text{h.c.} \end{aligned} \qquad (7)$$

Due to the general property $\mathbf{w}_M = -\sum_{j=1}^{M-1}\mathbf{w}_j$, the vectors appearing in the three exponents sum to zero, and hence a three-point correlator involving the product $S_1S_2S_3$ could survive. Since $\sigma_1\sigma_2\sigma_3 \sim 1_2$, the Pauli matrices also allow this to happen. These steps imply the three-point correlation function as quoted in Eq. (7) of the main text, where $\varepsilon_{jkl}$ arises due to the anticommutation property of the Pauli matrices. This result fulfills a number of consistency requirements: (i) The time dependence of the three-point correlator is what conformal invariance dictates [3, 4]. (ii) The presence of $\varepsilon_{jkl}$ is consistent with the SO(3) symmetry of the Kondo fixed point. (iii) The correlator is invariant under a simultaneous exchange of vector indices and time arguments. This is required since the three-point correlator is the functional derivative $\frac{\delta^3}{\delta h_j(\tau_1)\delta h_k(\tau_2)\delta h_l(\tau_3)}\mathcal{F}$ of the free energy $\mathcal{F}$ with respect to the conjugate Zeeman field $\boldsymbol{h}(\tau)$, and mixed derivatives commute.

To find how this generalizes for higher $M$, we first find sums of $\pm(\mathbf{w}_j + \mathbf{w}_k)$ that vanish. For odd $M$, we have

$$\begin{aligned} (\mathbf{w}_1 + \mathbf{w}_2) + (\mathbf{w}_2 + \mathbf{w}_3) + \ldots + (\mathbf{w}_M + \mathbf{w}_1) \\ = 2\sum_{j=1}^{M-1}\mathbf{w}_j - 2\sum_{j=1}^{M-1}\mathbf{w}_j = 0, \end{aligned} \qquad (8)$$

where we used $\mathbf{w}_M = -\sum_{j=1}^{M-1}\mathbf{w}_j$ again. The corresponding Majoranas multiply to the identity, $\gamma_1\gamma_2\ldots\gamma_M\gamma_1 = 1$. Hence the $M$-point function survives,

$$\begin{aligned} &\left\langle \mathcal{T}_\tau \mathcal{S}_{12}^{(+)}(\tau_1)\mathcal{S}_{23}^{(+)}(\tau_2)\ldots\mathcal{S}_{M-1,M}^{(+)}(\tau_{M-1})\mathcal{S}_{M,1}^{(+)}(\tau_M)\right\rangle \\ &\sim \frac{\text{sgn}(\tau_{12}\tau_{23}\ldots\tau_{M1})}{|\tau_{12}\tau_{23}\ldots\tau_{M1}|^{(4-M)/M}\prod'_{j<k}|\tau_{jk}|^{4/M}}, \end{aligned} \qquad (9)$$

where $\prod'$ is a product over the remaining time differences $\tau_{jk}$. However, the vanishing of the vector sum alone does not automatically lead to a surviving multi-point function. As an example, we consider the $M/2$-point correlator for even $M$, where we have the vanishing sum

$$\begin{aligned} (\mathbf{w}_1 + \mathbf{w}_2) + (\mathbf{w}_3 + \mathbf{w}_4) + \ldots + (\mathbf{w}_{M-1} + \mathbf{w}_M) = \\ \sum_{j=1}^{M-1}\mathbf{w}_j - \sum_{j=1}^{M-1}\mathbf{w}_j. \end{aligned} \qquad (10)$$

The Majorana factor is now $P_M = \gamma_1\gamma_2\gamma_3\ldots\gamma_M$. As this commutes with all parity products $p_jp_k$, it gives an

additional quantum number. In each $P_M = \pm$ sector, we get

$$\left\langle \mathcal{T}_\tau \mathcal{S}^{(+)}_{12}(\tau_1)\mathcal{S}^{(+)}_{34}(\tau_2)\dots\mathcal{S}^{(+)}_{M-1,M}(\tau_{M/2})\right\rangle \sim \frac{1}{\prod_{j<k}|\tau_{jk}|^{4/M}}. \quad (11)$$

Tracing over $P_M = \pm 1$ amounts to adding the same contribution but with opposite sign, and thus leads to a vanishing overall result. The $M/2$-point correlation function only survives for $M = M_{\rm tot}$, where $P_M$ represents the overall electron parity of the island and therefore only one $P_M = \pm$ sector is realized.

## CHARGE TRANSPORT

In this section, we study how to leading order the Zeeman field $h_{jk}$ interferes with charge transport near the Kondo fixed point. We shall focus on the linear conductance coefficients $G_{jk}$, where second-order perturbation theory produces the leading term. We have also explicitly verified that no third-order corrections to $G_{jk}$ are present, but here discuss only the second order. To this end, we consider the imaginary-time current-current correlation function, $C_{jk}(\omega_n) = \langle(\omega_n\varphi_{j,n})(-\omega_n\varphi_{k,-n})\rangle$, probing current flow in lead $j$ in linear response to a chemical potential variation in wire $k$. Here, $\omega_n$ are bosonic Matsubara frequencies, and $\varphi_{j,n}$ the corresponding field modes at the impurity position $x = 0$. From this function, the elements of the DC conductance tensor are obtained by standard analytic continuation, $G_{jk} = \frac{T}{2\pi}\lim_{\omega\to 0}\frac{1}{\omega^+}C_{jk}(\omega^+)$, where $\omega^+ = \omega + i0$. At lowest non-vanishing order in Zeeman field perturbation theory, we pick up a correction $C^{(2)}$, for which the functional expectation value has to be computed with an operator insertion $\langle(\dots)\rangle \to \langle(\dots)\frac{1}{T}\sum_{l<m}h^2_{lm}\int d\tau\, e^{iT\sum_n(\tilde\varphi_l+\tilde\varphi_m)_n(e^{-i\omega_n\tau}-e^{i\omega_n\tau})}\rangle_0$. Here, numerical constants are omitted, and the free boson field expectation value is $\langle\tilde\varphi_{j,n}\tilde\varphi_{k,-n'}\rangle_0 = T^{-1}C_n\delta_{nn'}Q_{jk}$ with $C_n = 4\pi/|\omega_n|$, where the matrix $Q_{jk}$ has been defined in the main text. Doing the Gaussian integrals over the $\tilde\varphi_j$ fields, we obtain

$$C^{(2)}_{jk} \sim \bar h^2 Z_{jk}\int d\tau\,(1-e^{i\omega_n\tau})e^{-\alpha(C(\tau)-C(0))}, \quad (12)$$

where $\alpha \equiv \frac{1}{2}(1-\frac{2}{M})$ and $Z_{jk} = \sum_{l\neq m}\frac{h^2_{lm}}{h^2}(Q_{jl}+Q_{jm})(Q_{lk}+Q_{mk})$. In computing the Fourier transform $C(\tau) = T\sum_n C_n e^{i\omega_n\tau}$, some care must be exercised not to miss analytic structures relevant to the correct evaluation of the conductance coefficients. By straightforward geometric series summation, we obtain $C(\tau)-C(0) = 4{\rm Re}\ln[(1-e^{2\pi iT\tau^+})\Lambda/2\pi T]$, where $\tau^+ = \tau + i\Lambda^{-1}$ and $\Lambda \sim T_K$ is a high-frequency cutoff. The subsequent integration over imaginary times is best done by deformation of the integration contour to two counter-propagating half-infinite *real* time contours, $\tau\to\epsilon - it$ and $\tau \to \beta-\epsilon-it$, with $t\in\mathbb{R}^+$ and $\epsilon$ positive infinitesimal. Substituting this parameterization into the integral, paying attention to the imaginary part of the logarithm along its cut, and limiting the time integration at $t\sim T$, we obtain the low-energy asymptotics in the form

$$C^{(2)}_{jk} \sim \bar h^2\omega_n Z_{jk}\sin\left(\frac{2\pi}{M}\right)\int_0^T dt\, t e^{-\alpha\ln(tT_K)}. \quad (13)$$

We finally perform the remaining elementary integral and analytically continue to real frequencies. In the end we arrive at Eq. (6) of the main text.

[1] A.O. Gogolin, A.A. Nersesyan, and A.M. Tsvelik, *Bosonization and strongly correlated systems* (Cambridge University Press, 1998).

[2] J. von Delft and H. Schoeller, Ann. Phys. (Berlin) **7**, 225 (1998).

[3] I. Affleck, Nucl. Phys. B **336**, 517 (1990); I. Affleck and A.W.W. Ludwig, Nucl. Phys. B **352**, 849 (1991); *ibid.* **360**, 641 (1991); *ibid.* **428**, 545 (1994).

[4] P. Di Francesco, P. Mathieu, and D. Sénéchal, *Conformal Field Theory* (Springer Verlag, New York, 1997).
